# Supplementary material for: Benchmarking Human and Automated Prompting in the Segment Anything Model
Source: arXiv:2410.22048 source file (2024-10-30)
Supplement: Supplementary file 1 [file AppendixC_Exterior.tex]

% Please add the following required packages to your document preamble:
% \usepackage{graphicx}
\begin{table}[H]
\caption{\textbf{Sampling Exclusion Points Far from Ground Truth Mask:} mIoU Results and Percent Change from Table \ref{tab:strategies-best}}
\label{tab:exterior}
\resizebox{\textwidth}{!}{%
\begin{tabular}{cccccccc}
\hline
\textbf{Category} & \textbf{Human mIoU}    & \textbf{Random mIoU} & \textbf{Saliency mIoU} & \textbf{K-Medoids mIoU}  & \textbf{Entropy mIoU} & \textbf{Maximum Dist mIoU} & \textbf{Shi-Tomasi mIoU} \\
\hline
\hline
Baseball bat  & \textbf{0.747 ± 0.152} & 0.681 (\textcolor{red}{$\downarrow$} -0.44\%) & 0.404 (\textcolor{red}{$\downarrow$} -4.27\%) & 0.722 (\textcolor{red}{$\downarrow$} -0.28\%) & 0.646 (\textcolor{red}{$\downarrow$} -1.07\%) & 0.623 (\textcolor{red}{$\downarrow$} -1.42\%) & 0.702 (\textcolor{green}{$\uparrow$} 0.14\%)  \\
Bird          & \textbf{0.677 ± 0.231} & 0.616 (\textcolor{green}{$\uparrow$} 0.16\%)  & 0.308 ( 0.00\%)                             & 0.647 (\textcolor{green}{$\uparrow$} 0.31\%)  & 0.483 ( 0.00\%)                             & 0.44 (\textcolor{red}{$\downarrow$} -3.51\%)  & 0.614 (\textcolor{red}{$\downarrow$} -0.97\%) \\
Bus           & \textbf{0.803 ± 0.144} & 0.579 (\textcolor{red}{$\downarrow$} -2.36\%) & 0.149 (\textcolor{red}{$\downarrow$} -5.70\%) & 0.632 (\textcolor{red}{$\downarrow$} -0.63\%) & 0.341 (\textcolor{red}{$\downarrow$} -5.01\%) & 0.268 (\textcolor{red}{$\downarrow$} -7.27\%) & 0.528 (\textcolor{red}{$\downarrow$} -3.65\%) \\
Cat           & \textbf{0.887 ± 0.079} & 0.767 (\textcolor{red}{$\downarrow$} -0.52\%) & 0.484 (\textcolor{red}{$\downarrow$} -0.62\%) & 0.823 (\textcolor{red}{$\downarrow$} -0.24\%) & 0.571 (\textcolor{red}{$\downarrow$} -2.06\%) & 0.485 (\textcolor{red}{$\downarrow$} -4.53\%) & 0.786 (\textcolor{red}{$\downarrow$} -1.13\%) \\
Clock         & \textbf{0.814 ± 0.181} & 0.749 (\textcolor{green}{$\uparrow$} 0.54\%)  & 0.424 (\textcolor{red}{$\downarrow$} -1.85\%) & 0.74 (\textcolor{green}{$\uparrow$} 0.68\%)   & 0.685 (\textcolor{green}{$\uparrow$} 0.74\%)  & 0.693 (\textcolor{green}{$\uparrow$} 0.14\%)  & 0.711 (\textcolor{red}{$\downarrow$} -0.56\%) \\
Cow           & \textbf{0.808 ± 0.130} & 0.66 (\textcolor{red}{$\downarrow$} -2.22\%)  & 0.32 (\textcolor{red}{$\downarrow$} -0.31\%)  & 0.642 (\textcolor{red}{$\downarrow$} -2.73\%) & 0.404 (\textcolor{red}{$\downarrow$} -4.49\%) & 0.322 (\textcolor{red}{$\downarrow$} -6.12\%) & 0.614 (\textcolor{red}{$\downarrow$} -4.95\%) \\
Dog           & \textbf{0.848 ± 0.102} & 0.731 (\textcolor{red}{$\downarrow$} -1.48\%) & 0.443 (\textcolor{green}{$\uparrow$} 1.61\%)  & 0.779 (\textcolor{red}{$\downarrow$} -0.13\%) & 0.539 (\textcolor{red}{$\downarrow$} -0.92\%) & 0.511 (\textcolor{red}{$\downarrow$} -2.29\%) & 0.73 (\textcolor{red}{$\downarrow$} -2.01\%)  \\
Tie           & \textbf{0.700 ± 0.276} & 0.63 (\textcolor{green}{$\uparrow$} 0.48\%)   & 0.372 (\textcolor{green}{$\uparrow$} 1.09\%)  & 0.649 ( 0.00\%)                             & 0.566 (\textcolor{red}{$\downarrow$} -0.53\%) & 0.535 (\textcolor{red}{$\downarrow$} -1.29\%) & 0.649 (\textcolor{green}{$\uparrow$} 0.46\%)  \\
Stop sign     & \textbf{0.886 ± 0.132} & 0.834 (\textcolor{red}{$\downarrow$} -0.60\%) & 0.537 (\textcolor{red}{$\downarrow$} -2.36\%) & 0.851 (\textcolor{green}{$\uparrow$} 0.35\%)  & 0.755 (\textcolor{red}{$\downarrow$} -2.33\%) & 0.723 (\textcolor{red}{$\downarrow$} -0.41\%) & 0.615 (\textcolor{red}{$\downarrow$} -3.91\%) \\
Dolphin above & \textbf{0.732 ± 0.100} & 0.639 (\textcolor{red}{$\downarrow$} -0.47\%) & 0.464 (\textcolor{red}{$\downarrow$} -1.69\%) & 0.655 ( 0.00\%)                             & 0.548 (\textcolor{red}{$\downarrow$} -0.90\%) & 0.521 (\textcolor{red}{$\downarrow$} -4.05\%) & 0.654 (\textcolor{red}{$\downarrow$} -1.06\%) \\
Dolphin below & \textbf{0.831 ± 0.075} & 0.658 (\textcolor{red}{$\downarrow$} -1.79\%) & 0.385 (\textcolor{red}{$\downarrow$} -1.53\%) & 0.71 (\textcolor{red}{$\downarrow$} -0.56\%)  & 0.453 (\textcolor{red}{$\downarrow$} -4.23\%) & 0.397 (\textcolor{red}{$\downarrow$} -7.67\%) & 0.665 (\textcolor{red}{$\downarrow$} -2.35\%) \\
Polyp         & \textbf{0.794 ± 0.145} & 0.746 (\textcolor{red}{$\downarrow$} -0.13\%) & 0.544 (\textcolor{red}{$\downarrow$} -0.55\%) & 0.76 (\textcolor{green}{$\uparrow$} 0.40\%)   & 0.64 (\textcolor{green}{$\uparrow$} 0.95\%)   & 0.451 (\textcolor{green}{$\uparrow$} 8.67\%)  & 0.618 (\textcolor{red}{$\downarrow$} -2.98\%) \\
Skin          & 0.593 ± 0.195          & 0.593 ( 0.00\%)                             & 0.382 (\textcolor{green}{$\uparrow$} 1.87\%)  & \textbf{0.634} (\textcolor{green}{$\uparrow$} 1.28\%)  & 0.463 (\textcolor{green}{$\uparrow$} 2.43\%)  & 0.387 (\textcolor{red}{$\downarrow$} -2.03\%) & 0.493 (\textcolor{red}{$\downarrow$} -4.27\%) \\
Breast        & \textbf{0.750 ± 0.126} & 0.626 (\textcolor{green}{$\uparrow$} 0.81\%)  & 0.45 (\textcolor{green}{$\uparrow$} 2.74\%)   & 0.682 (\textcolor{green}{$\uparrow$} 1.19\%)  & 0.577 (\textcolor{green}{$\uparrow$} 1.94\%)  & 0.515 (\textcolor{red}{$\downarrow$} -3.20\%) & 0.585 (\textcolor{red}{$\downarrow$} -1.18\%) \\
Salt dome     & \textbf{0.844 ± 0.096} & 0.514 (\textcolor{green}{$\uparrow$} 0.19\%)  & 0.278 (\textcolor{green}{$\uparrow$} 1.83\%)  & 0.607 (\textcolor{green}{$\uparrow$} 3.23\%)  & 0.367 (\textcolor{green}{$\uparrow$} 5.76\%)  & 0.3 (\textcolor{red}{$\downarrow$} -1.96\%)   & 0.567 (\textcolor{green}{$\uparrow$} 0.53\%)  \\
Chalk group   & \textbf{0.714 ± 0.101} & 0.387 (\textcolor{red}{$\downarrow$} -5.38\%) & 0.242 (\textcolor{green}{$\uparrow$} 2.11\%)  & 0.403 (\textcolor{red}{$\downarrow$} -8.62\%) & 0.305 (\textcolor{red}{$\downarrow$} -0.97\%) & 0.288 (\textcolor{red}{$\downarrow$} -3.68\%) & 0.402 (\textcolor{red}{$\downarrow$} -5.41\%)\\
\hline
\end{tabular}%
}
\end{table}
