# Supplementary material for: Benchmarking Human and Automated Prompting in the Segment Anything Model
Source: arXiv:2410.22048 source file (2024-10-30)
Supplement: Supplementary file 2 [file AppendixC_Perim.tex]

% Please add the following required packages to your document preamble:
% \usepackage{graphicx}
\begin{table}[H]
\caption{\textbf{Sampling Exclusion Points Near Perimeter of Ground Truth Mask}: mIoU Results and Percent Change from Table \ref{tab:strategies-best}}
\label{tab:perimeter}
\resizebox{\textwidth}{!}{%
\begin{tabular}{cccccccc}
\hline
\textbf{Category} & \textbf{Human mIoU}   & \textbf{Random mIoU} & \textbf{Saliency mIoU} & \textbf{K-Medoids mIoU}  & \textbf{Entropy mIoU} & \textbf{Maximum Dist mIoU} & \textbf{Shi-Tomasi mIoU} \\
\hline
\hline
Baseball bat  & \textbf{0.747 ± 0.152} & 0.667 (\textcolor{red}{$\downarrow$} -2.49\%)  & 0.314 (\textcolor{red}{$\downarrow$} -25.59\%) & 0.72 (\textcolor{red}{$\downarrow$} -0.55\%)   & 0.631 (\textcolor{red}{$\downarrow$} -3.37\%)  & 0.587 (\textcolor{red}{$\downarrow$} -7.12\%)  & 0.691 (\textcolor{red}{$\downarrow$} -1.43\%)  \\
Bird          & \textbf{0.677 ± 0.231} & 0.609 (\textcolor{red}{$\downarrow$} -0.98\%)  & 0.282 (\textcolor{red}{$\downarrow$} -8.44\%)  & 0.642 (\textcolor{red}{$\downarrow$} -0.47\%)  & 0.463 (\textcolor{red}{$\downarrow$} -4.14\%)  & 0.389 (\textcolor{red}{$\downarrow$} -14.69\%) & 0.61 (\textcolor{red}{$\downarrow$} -1.61\%)   \\
Bus           & \textbf{0.803 ± 0.144} & 0.56 (\textcolor{red}{$\downarrow$} -5.56\%)   & 0.147 (\textcolor{red}{$\downarrow$} -6.96\%)  & 0.61 (\textcolor{red}{$\downarrow$} -4.09\%)   & 0.314 (\textcolor{red}{$\downarrow$} -12.53\%) & 0.217 (\textcolor{red}{$\downarrow$} -24.91\%) & 0.506 (\textcolor{red}{$\downarrow$} -7.66\%)  \\
Cat           & \textbf{0.887 ± 0.079} & 0.755 (\textcolor{red}{$\downarrow$} -2.08\%)  & 0.477 (\textcolor{red}{$\downarrow$} -2.05\%)  & 0.817 (\textcolor{red}{$\downarrow$} -0.97\%)  & 0.535 (\textcolor{red}{$\downarrow$} -8.23\%)  & 0.408 (\textcolor{red}{$\downarrow$} -19.69\%) & 0.776 (\textcolor{red}{$\downarrow$} -2.39\%)  \\
Clock         & \textbf{0.814 ± 0.181} & 0.703 (\textcolor{red}{$\downarrow$} -5.64\%)  & 0.354 (\textcolor{red}{$\downarrow$} -18.06\%) & 0.703 (\textcolor{red}{$\downarrow$} -4.35\%)  & 0.618 (\textcolor{red}{$\downarrow$} -9.12\%)  & 0.628 (\textcolor{red}{$\downarrow$} -9.25\%)  & 0.669 (\textcolor{red}{$\downarrow$} -6.43\%)  \\
Cow           & \textbf{0.808 ± 0.130} & 0.644 (\textcolor{red}{$\downarrow$} -4.59\%)  & 0.308 (\textcolor{red}{$\downarrow$} -4.05\%)  & 0.633 (\textcolor{red}{$\downarrow$} -4.09\%)  & 0.389 (\textcolor{red}{$\downarrow$} -8.04\%)  & 0.286 (\textcolor{red}{$\downarrow$} -16.62\%) & 0.605 (\textcolor{red}{$\downarrow$} -6.35\%)  \\
Dog           & \textbf{0.848 ± 0.102} & 0.712 (\textcolor{red}{$\downarrow$} -4.04\%)  & 0.414 (\textcolor{red}{$\downarrow$} -5.05\%)  & 0.762 (\textcolor{red}{$\downarrow$} -2.31\%)  & 0.496 (\textcolor{red}{$\downarrow$} -8.82\%)  & 0.427 (\textcolor{red}{$\downarrow$} -18.36\%) & 0.711 (\textcolor{red}{$\downarrow$} -4.56\%)  \\
Tie           & \textbf{0.700 ± 0.276} & 0.621 (\textcolor{red}{$\downarrow$} -0.96\%)  & 0.302 (\textcolor{red}{$\downarrow$} -17.93\%) & 0.647 (\textcolor{red}{$\downarrow$} -0.31\%)  & 0.543 (\textcolor{red}{$\downarrow$} -4.57\%)  & 0.478 (\textcolor{red}{$\downarrow$} -11.81\%) & 0.64 (\textcolor{red}{$\downarrow$} -0.93\%)   \\
Stop sign     & \textbf{0.886 ± 0.132} & 0.829 (\textcolor{red}{$\downarrow$} -1.19\%)  & 0.49 (\textcolor{red}{$\downarrow$} -10.91\%)  & 0.845 (\textcolor{red}{$\downarrow$} -0.35\%)  & 0.738 (\textcolor{red}{$\downarrow$} -4.53\%)  & 0.641 (\textcolor{red}{$\downarrow$} -11.71\%) & 0.592 (\textcolor{red}{$\downarrow$} -7.50\%)  \\
Dolphin above & \textbf{0.732 ± 0.100} & 0.625 (\textcolor{red}{$\downarrow$} -2.65\%)  & 0.407 (\textcolor{red}{$\downarrow$} -13.77\%) & 0.646 (\textcolor{red}{$\downarrow$} -1.37\%)  & 0.536 (\textcolor{red}{$\downarrow$} -3.07\%)  & 0.507 (\textcolor{red}{$\downarrow$} -6.63\%)  & 0.644 (\textcolor{red}{$\downarrow$} -2.57\%)  \\
Dolphin below & \textbf{0.831 ± 0.075} & 0.688 (\textcolor{green}{$\uparrow$} 2.69\%)   & 0.392 (\textcolor{green}{$\uparrow$} 0.26\%)   & 0.716 (\textcolor{green}{$\uparrow$} 0.28\%)   & 0.513 (\textcolor{green}{$\uparrow$} 8.46\%)   & 0.404 (\textcolor{red}{$\downarrow$} -6.05\%)  & 0.691 (\textcolor{green}{$\uparrow$} 1.47\%)   \\
Polyp         & \textbf{0.794 ± 0.145} & 0.738 (\textcolor{red}{$\downarrow$} -1.20\%)  & 0.544 (\textcolor{red}{$\downarrow$} -0.55\%)  & 0.751 (\textcolor{red}{$\downarrow$} -0.79\%)  & 0.613 (\textcolor{red}{$\downarrow$} -3.31\%)  & 0.403 (\textcolor{red}{$\downarrow$} -2.89\%)  & 0.604 (\textcolor{red}{$\downarrow$} -5.18\%)  \\
Skin          & 0.593 ± 0.195          & 0.591 (\textcolor{red}{$\downarrow$} -0.34\%)  & 0.384 (\textcolor{green}{$\uparrow$} 2.40\%)   & \textbf{0.627} (\textcolor{green}{$\uparrow$} 0.16\%)   & 0.442 (\textcolor{red}{$\downarrow$} -2.21\%)  & 0.328 (\textcolor{red}{$\downarrow$} -16.96\%) & 0.497 (\textcolor{red}{$\downarrow$} -3.50\%)  \\
Breast        & \textbf{0.750 ± 0.126} & 0.611 (\textcolor{red}{$\downarrow$} -1.61\%)  & 0.4 (\textcolor{red}{$\downarrow$} -8.68\%)    & 0.671 (\textcolor{red}{$\downarrow$} -0.45\%)  & 0.541 (\textcolor{red}{$\downarrow$} -4.42\%)  & 0.472 (\textcolor{red}{$\downarrow$} -11.28\%) & 0.574 (\textcolor{red}{$\downarrow$} -3.04\%)  \\
Salt dome     & \textbf{0.844 ± 0.096} & 0.488 (\textcolor{red}{$\downarrow$} -4.87\%)  & 0.212 (\textcolor{red}{$\downarrow$} -22.34\%) & 0.578 (\textcolor{red}{$\downarrow$} -1.70\%)  & 0.295 (\textcolor{red}{$\downarrow$} -14.99\%) & 0.248 (\textcolor{red}{$\downarrow$} -18.95\%) & 0.529 (\textcolor{red}{$\downarrow$} -6.21\%)  \\
Chalk group   & \textbf{0.714 ± 0.101} & 0.296 (\textcolor{red}{$\downarrow$} -27.63\%) & 0.187 (\textcolor{red}{$\downarrow$} -21.10\%) & 0.357 (\textcolor{red}{$\downarrow$} -19.05\%) & 0.299 (\textcolor{red}{$\downarrow$} -2.92\%)  & 0.257 (\textcolor{red}{$\downarrow$} -14.05\%) & 0.317 (\textcolor{red}{$\downarrow$} -25.41\%) \\
\hline
\end{tabular}%
}
\end{table}
